# Supplementary material for: Holographic Beam Measurements of the Canadian Hydrogen Intensity Mapping Experiment (CHIME)
Source: arXiv:2408.00172 source file (2024-07-31)
Supplement: Supplementary file 1 [file appendices.tex]

\appendix
